# Supplementary material for: A Probabilistic Fluctuation based Membership Inference Attack for Diffusion Models
Source: arXiv:2308.12143 source file (2024-12-26)
Supplement: Supplementary file 1 [file 7.Appendix.tex]

\clearpage
% \onecolumn
\appendix
% \linespread{1}
\section{Appendix}

% \subsubsection{Text}

% \begin{table}
% \centering
% \caption{Performance of xxx on the text generation task with different perturbation techniques.}
% \resizebox{\linewidth}{!}{%
% \begin{tabular}{c|cclcc} 
% \hline
% Perturbation Techniques & ASR   & AUC   & TPR @ 1\textbackslash{}\% FPR & $Var_{mem}$ & $Var_{/mem}$  \\ 
% \hline
% Synonym Replacement     & 0.888 & 0.888 &                               & $33\%$    & $13\%$      \\ 
% \hline
% Random Insertation      &       &       &                               &           &             \\ 
% \hline
% Random Swap             &       &       &                               &           &             \\ 
% \hline
% Random Deletion         &       &       &                               &           &             \\
% \hline
% \end{tabular}
% }
% \end{table}

% \section{Detailed Configurations of Baselines}
